# Supplementary material for: Policy Synthesis for Metric Interval Temporal Logic with Probabilistic Distributions
Source: arXiv:2105.04593 source file (2021-05-10)
Supplement: Supplementary file 1 [file appendix.tex]

\appendix
